# Supplementary material for: The Graph Database Interface: Scaling Online Transactional and Analytical Graph Workloads to Hundreds of Thousands of Cores
Source: arXiv:2305.11162 source file (2023-11-20)
Supplement: Supplementary file 1 [file appendix.tex]

\section{GDI Listing Summary}

\input{gdi-listing.tex}

%\input{gdi-list-table.tex}
